# Supplementary material for: Federated Learning with Flexible Architectures
Source: arXiv:2406.09877 source file (2024-06-14)
Supplement: Supplementary file 1 [file appendix_filter_grafting.tex]

\newpage
\clearpage
\section{Analysis of Filter Grafting Efficacy} \label{apdx: filter grafting}
\begin{algorithm}[ht]
\caption{Filter Grafting Procedure. Local model $M_c$ refers to the local model of client $c$. For the layer with index $l$, $N_{width,\max}^{(l)}$ denotes the maximum layer width across clients. $N_{width,c}^{(l)}$ is the current width of layer $M_c^{(l)}$ of client $c$, while $\Delta W$ represents the width difference that needs to be augmented. $||M_k^{(l)}||_2$ represents the \textit{importance} of the $k$-th filter in layer $M_c^{(l)}$, and $\oplus$ denotes the grafting operation. The algorithm ensures that the width of each layer $M_c^{(l)}$ matches $N_{width,\max}^{(l)}$, through selective filter grafting based on filter importance.}
\label{algorithm: filter grafting}
\begin{algorithmic}[1]
\REQUIRE Local model $M_c$ of client $c$, maximum layer width $N_{width,\max}^{(l)}$ for the layer index $l$ across all clients.
\ENSURE Updated local model $M_c$ with grafted filters matching $N_{width,\max}^{(l)}$.
\FOR{each layer $M_c^{(l)}$ in model $M_c$}
    \STATE $N_{width,c}^{(l)} \gets \text{current width of layer } M_c^{(l)}$
    \STATE $\Delta W \gets N_{width,\max}^{(l)} - N_{width,c}^{(l)}$
    \IF{$\Delta W > 0$}
        \STATE Compute importance $||M_k^{(l)}||_2$ for each filter $k$
        \STATE $\text{Indices}_{\text{Top}} \gets \text{indices of top } \Delta W \text{ filters by } |M_k^{(l)}|$
        \STATE Expand layer $M_c^{(l)}$ by grafting top filters: \\
        $M_c^{(l)} \gets M_c^{(l)} \oplus M_c^{(l)}[\text{Indices}_{\text{Top}}]$
        \FOR{each filter $M_k^{(l+1)}$ in layer $M_c^{(l+1)}$}
            \STATE $M_k^{(l+1)} \gets M_k^{(l+1)} \oplus M_k^{(l+1)}[\text{Indices}_{\text{Top}}]$
        \ENDFOR
    \ENDIF
\ENDFOR
\end{algorithmic}
\end{algorithm}

\subsection{Mathematical Framework for Filter Grafting}
Filter grafting in Federated Learning can be understood as a process analogous to pruning but with an emphasis on replication and reinforcement of crucial filters. This approach aims to amplify the impact of significant filters in each layer, thereby improving the model's performance and efficiency. To analyze this, we consider the contribution of individual filters to the output of a layer and the overall network's performance.

Let's denote the set of filters in the $l$ layer of a network by $\{M_k^{(l)}\}_{k=1}^{N_l}$, where $N_l$ is the number of filters in the layer. The importance of each filter can be quantified by a metric such as the norm of the filter weights, $||M_k^{(l)}||$. Filters with higher norms are considered more significant in contributing to the network's performance. 

The output of the $l$ layer, before activation, for an input $x$ can be expressed as:
\[
Z^{(l)}(x) = \sum_{k=1}^{N_l} x * M_k^{(l)}
\]
where $*$ denotes the convolution operation.

In filter grafting, we replicate filters with the highest norms. If we replicate the top $M$ filters, the new set of filters becomes $\{M_k^{(l)}, M_{k'}^{(l)}\}_{k=1, k'=1}^{N_l, M}$, where $M_{k'}^{(l)}$ is a copy of the $k'$-th most important filter. The modified output of the layer can be represented as:
\[
Z_{\text{aug}}^{(l)}(x) = \sum_{k=1}^{N_l} x * M_k^{(l)} + \sum_{k'=1}^{M} x * M_{k'}^{(l)}
\]

\subsection{Efficacy of Filter Grafting}
The efficacy of filter grafting can be analyzed through its impact on the layer's output and, consequently, on the network's learning and generalization capabilities. The replication of critical filters amplifies their contribution to the output, potentially enhancing the layer's ability to capture relevant features in the input data.

\subsubsection{Enhanced Feature Representation}
By doubling the contribution of the most significant filters, filter grafting enhances the representation of crucial features. This is particularly beneficial in scenarios where the dataset exhibits high variability or complexity, as the amplified filters are better positioned to capture essential patterns with secure aggregation.

\subsubsection{Comparison with Pruning}
Pruning and filter grafting represent two sides of the same coin in terms of their impact on model architecture. While pruning reduces model complexity by selectively removing less significant filters, filter grafting increases the dominance of important filters without reducing the network's capacity. This can be particularly advantageous in FL, where client-specific models might require maintaining a certain level of complexity to effectively learn from diverse local datasets.

To mathematically compare these approaches, consider a simplified model where the output of a layer is a linear combination of its filter responses. For a given layer with $N$ filters, let's denote the set of filters as $\{M_k\}_{k=1}^{N}$ and their corresponding importance scores as $\{s_k\}_{k=1}^{N}$, where higher $s_k$ indicates more importance.

\textbf{Pruning:} In pruning, we remove a proportion of filters with the lowest importance scores. Let's denote the number of filters to be pruned as $P$. The pruned output can be represented as:
\[
Z_{\text{pruned}} = \sum_{k=P+1}^{N} x * M_k
\]
Here, the first $P$ filters with the lowest importance scores are removed.

\textbf{Filter Grafting:} In contrast, filter grafting duplicates the most important filters. If we replicate the top $M$ filters, the augmented layer's output becomes:
\[
Z_{\text{aug}} = \sum_{k=1}^{N} x * M_k + \sum_{k'=1}^{M} x * M_{k'}
\]
where $M_{k'}$ is a copy of the $k'$-th most important filter.

\textbf{Dominance of Important Filters:} Both pruning and filter grafting aim to emphasize the contribution of significant filters. In pruning, the removal of less important filters naturally increases the relative importance of the remaining ones. In filter grafting, duplicating important filters directly amplifies their influence. The augmented output due to grafting can be viewed as an intensified focus on the features captured by the most crucial filters.

\textbf{Implications:} Both techniques alter the learning dynamics of the network, but filter grafting does so by enhancing rather than reducing the network's capacity. This can be especially beneficial in FL environments, allowing client models to retain their complexity while still focusing on the most effective features for learning from their local datasets.

In summary, while pruning and filter grafting employ different strategies, their underlying goal is similar: to optimize the network's focus on the most important features. Filter grafting achieves this not by removing but by reinforcing the influence of crucial filters, aligning well with the diverse and decentralized nature of FL.

\subsubsection{Impact on Learning Dynamics}
The augmented filters in filter grafting can alter the learning dynamics of the network. The reinforced filters dominate the gradient flow during backpropagation, potentially leading to faster convergence on crucial features and improved model robustness against overfitting to less relevant patterns.

\subsection{Summary}
Through a mathematical analysis, we demonstrate that filter grafting effectively enhances the influence of critical filters in a network, akin to emphasizing the most informative features in pruning. This approach aligns well with the objectives of FL, offering a nuanced method to optimize network architectures across diverse client datasets. Filter grafting not only preserves the model's capacity but also ensures that key features are adequately represented, contributing to improved learning outcomes and model generalization.
